# Supplementary material for: Graph-based multimodal multi-lesion DLBCL treatment response prediction from PET images
Source: arXiv:2310.16863 source file (2023-10-25)
Supplement: Supplementary file 1 [file AI4TREAT_supp_material-2.pdf]

**Table 1.** Lesions imaging features

| Classical features | Radiomics | |
|---|---|---|
| Standard uptake value of the maximum intensity voxel inside the lesion (SUVmax) | Shape | Sphericity |
| Metabolic Tumor Volume (MTV) of the lesion | Second order | Contrast |
| Total lesion glycolysis (TLG) from each of the segmented lesions | | Correlation |
| Mean intensity | | Inverse difference normalized |
| Standard deviation of intensity | | Joint energy |
| Entropy of intensity | | |

**Table 2.** Clinical features considered in the study

| Name | Explaination |
|---|---|
| Age | The higher it is, the higher the risk for the patient. |
| Lactate dehydrogenase (LDH) | An enzyme present in cells used as a biomarker for DLBCL diagnosis and prognosis. |
| Categorical LDH | Whether the LDH level is higher than it should be, the expected value depending on the measurement process. |
| Ann Arbor stage | Ranges from 1 to 4 depending on where the malignant tissues are located. |
| Number of extranodal sites | Having more than one extranodal site of involvement is usually an indication of a poor prognosis. |
| ECOG scale | Ranges from 0 to 5 and describes a patient's ability to take care of themselves and perform daily activities. |
| Age-adjusted IPI (aaIPI) | Classifies the DLBCL patients into four risk groups (0 to 3), based on 3 factors: (a) performance status - a score determining thepatient's ability to perform certain day-to-day activities, (b) stage and (c) LDH level. |
| Treatment type | Course of treatment administered to the patient: chemoterapy regimen, autologous cell transplant or salvage therapy (which are considered as three different binary variables). |

**Table 3.** Baselines configuration (HC = hidden channels ; LR = learning rate)

| Model | Search space | Best parameters | Number of epochs |
|---|---|---|---|
| MLP clinical | HC: {16, 32, 64, 128}<br>LR: {0.1, 0.01, 0.001, 0.0001} | HC=16<br>LR=0.01 | 100 |
| MLP clinical+image | HC: {16, 32, 64, 128}<br>LR: {0.1, 0.01, 0.001, 0.0001} | HC=128<br>LR=0.01 | 100 |
| MLP image | HC: {16, 32, 64, 128}<br>LR: {0.1, 0.01, 0.001, 0.0001} | HC=128<br>LR=0.01 | 500 |
| MIL image | HC: {16, 32, 64, 128}<br>LR: {0.1, 0.01, 0.001, 0.0001} | HC=16<br>LR=0.01 | 500 |
| GraphConv image | HC: {16, 32, 64, 128}<br>LR: {0.01, 0.001, 0.0001, 1e-05}<br>$\alpha$: {0.1, 1, 10, 50} | HC=32<br>LR=0.01<br>$\alpha$=0.1 | 500 |

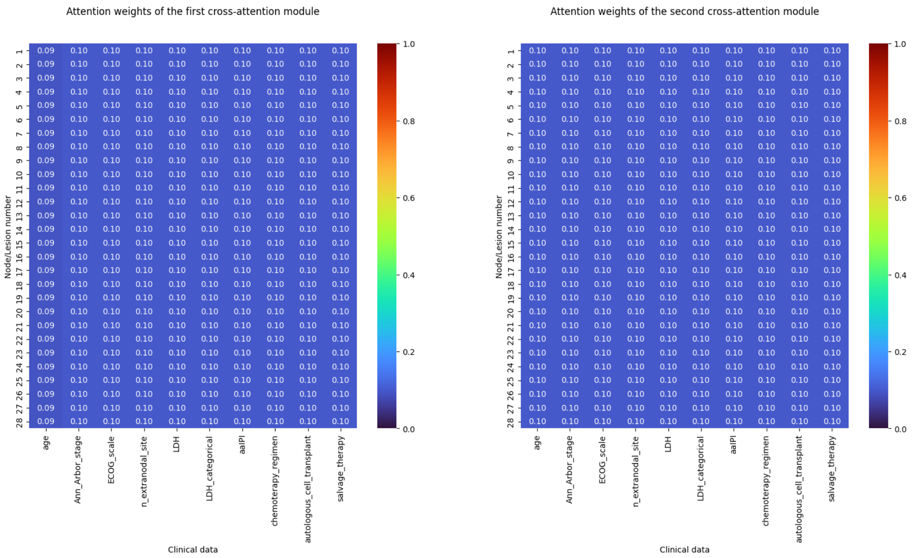


**Fig. 1.** Attention weights of a patient with fully constant weights

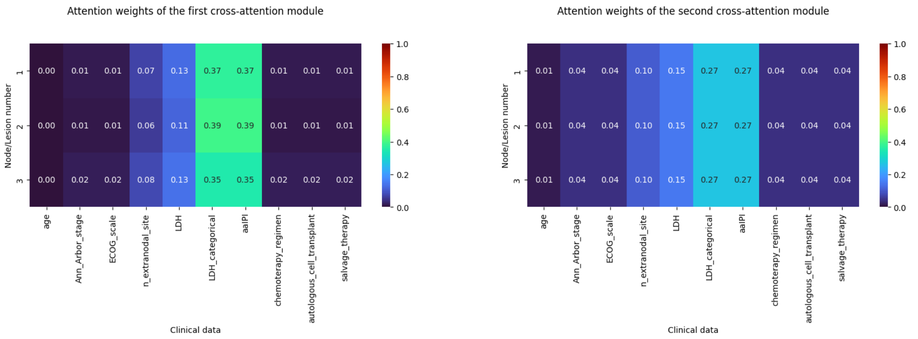


**Fig. 2.** Attention weights of a patient with stable clinical weights relatively to the nodes

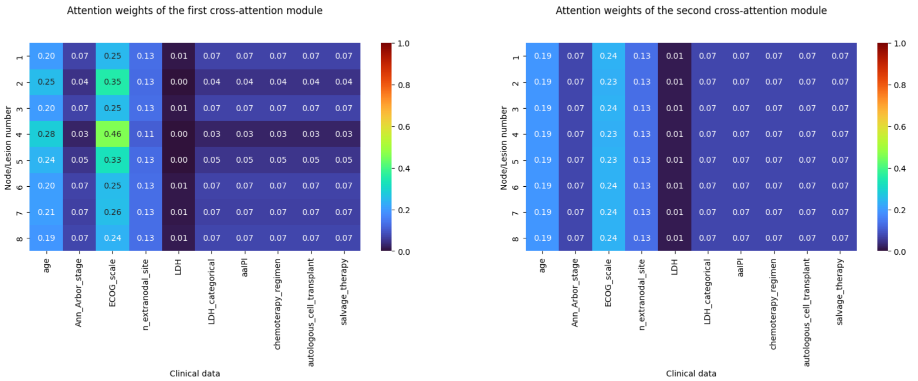


**Fig. 3.** Attention weights of a patient with more diverse node/clinical weights
